# Supplementary material for: TE2Rules: Explaining Tree Ensembles using Rules
Source: arXiv:2206.14359 source file (2024-01-23)
Supplement: Supplementary file 1 [file appendix.tex]

\section*{Appendix}
\appendix

%\section{Reproducibility}
%Here is our (anonymized) code implementing TE2Rules: \url{https://anonymous.4open.science/r/TE2Rules-AAAI24/}. The code has a Readme file with instructions on how to reproduce the plots presented in this paper. We are happy to share our original unanonymous implementation, once our work is accepted.  

\section{Reproducibility}
Here is our code implementing TE2Rules: \url{https://github.com/linkedin/TE2Rules}. The code has a Readme file with instructions on how to reproduce the plots presented in this paper. 

\section{Psudocode of TE2Rules}
In this section we present a pseudocode of TE2Rules. Algorithm \ref{alg:te2rules} shows the overall sketch of TE2Rules. It makes references to various helper methods. Pseudocode of the helper functions are also given below. TE2Rules algorithm runs in two phase: Rule Generation and Rule Simplification.

\begin{algorithm}
\caption{TE2Rules}\label{alg:te2rules}
\begin{algorithmic}

\State $solutions \gets []$
\\ \Comment{Rule Generation}
\For{$k \gets 1, 2, 3, \ldots n$}  
    \If{$k = 1$}
    \State $candidates \gets getNodeRules(model)$
    \Else
    \State $candidates \gets getNextStage(candidates, k)$  
    \EndIf
    \\
    \For{$r \gets candidates$}   
        \State $p \gets getPrecision(r \implies positiveLabel)$
        \If{$p > 1 - \delta$}
            \State $candidates.remove(r)$
            \State $solutions.append(r)$
        \EndIf
    \EndFor
\EndFor
\\ \Comment{Rule Simplification}
\State $solutions \gets greedySetCover(solutions)$
\\
\Return $solutions$

\end{algorithmic}
\end{algorithm}

The Rule Generation phase generates candidate rules for each stage and mines solution rules out of the candidates. For each candidate rule, we check if the rule formed by $candidate rule \implies positive$ agrees with the model prediction with high precision. Any candidate rule that has precision above $1 - \delta$ is promoted to be a solution rule. However, the generation phase can produce a lot of such solution rules. The Simplification stage selects a small subset of the solution rules that are effective in explaining the TE model and are easy for a human to comprehend with less number of rules.
\begin{algorithm}
\caption{getNodeRules(model)}\label{alg:te2rules_stage1}
\begin{algorithmic}

\State $candidates \gets []$
\\
\For{$tree \gets model$}    
    \For{$node \gets tree$}    
        \State $r \gets node.getDecisionPath()$
        \State $r.sourceNodes \gets [node]$
        \If{$|r.support| > \epsilon$}
            \State $candidates.append(r)$
        \EndIf
    \EndFor
\EndFor
\\
\Return $candidates$
\end{algorithmic}
\end{algorithm}

TE2Rules proceeds in stages and in stage-k, it explores all rules formed out of k-node combinations from the tree ensemble. For generating candidate rules, we use two helper methods: $getNodeRules()$ for the TE model for stage-1 candidates and $getNextStage()$ for any stage-k candidates (for all k >  $1$). $getNodeRules()$ is described in Algorithm \ref{alg:te2rules_stage1} and $getNextStage()$ is described in Algorithm \ref{alg:te2rules_stagek}. $getNodeRules()$ goes through every node in the tree ensemble and spits out the rule corresponding to the decision path to reach that node from its respective root node. Thus, it finds all individual nodes (or 1-node) combinations from the tree ensemble. It the filters out all rules which has very little (less than $epsilon$) support in data. $getNextStage()$ uses the candidates found in the previous stage to efficiently find the next stage candidates. It considers all pairs of candidates from stage-$k-1$ such that they share $k-2$ nodes in common. When such a pair of rules is combined (using logical and), they get a total of $(k-1) + (k-1) - (k-2) = k$ nodes as their source. It then filters out all rules which has very little (less than $epsilon$) support in data.

\begin{algorithm}
\caption{getNextStage(candidates, k)}\label{alg:te2rules_stagek}
\begin{algorithmic}

\State $newCandidates \gets []$  
\\
\For{$r_1 \gets candidates$}   
    \For{$r_2 \gets candidates$}   
        \State $nodes_1 = r_1.sourceNodes$
        \State $nodes_2 = r_2.sourceNodes$
        \If{$|nodes_1 \cap nodes_2| = k - 2$}
            \State $r \gets r_1 \& r_2$
            \State $r.sourceNodes \gets n_1 \cup n_2$
            \If{$|r.support| > \epsilon$}
                \State $candidates.append(r)$
            \EndIf
        \EndIf
    \EndFor
    \EndFor
\\
\Return $newCandidates$
\end{algorithmic}
\end{algorithm}

Generating stage $k$ candidates in this way, we make sure that we do not explore $k$ node combinations which can be proven to have little support ($< \epsilon$) using the node combinations already explored in stage $k-1$. Let us say there exists a $k$ node combination that can not be generated by the above process. Then, consider the $k-1$ node combinations formed out of the first $k-1$ nodes and the last $k-1$ nodes from the $k$ nodes. These two $k-1$ node combinations share $k-2$ common nodes. If both these node combinations were present among stage $k-1$ candidates, then they could be merged to form the $k$ nodes in stage $k$, by the above process. Hence, at least one of these two $k-1$ node combinations do not exist among stage $k-1$ candidate rules. This implies that at least one of the two $k-1$ node combinations has support $< \epsilon$. Thus, any $k$ node combinations containing the $k-1$ nodes would also have support $< \epsilon$ and is not worth considering in stage $k$.

\begin{algorithm}
\caption{greedySetCover(solutions)}\label{alg:te2rules_simplification}
\begin{algorithmic}

\State $newSolutions \gets []$
\State $cover \gets \phi$
\\
\While{$cover \neq allPositives$}
    \State{$r \gets maxPositiveCoverage(solutions)$}
    \State{$solutions.remove(r)$}
    \State{$newSolutions.append(r)$}
    \State{$cover \gets cover \cup r.coveredPositives$}
    
\EndWhile
\\
\Return $newSolutions$

\end{algorithmic}
\end{algorithm}

The generation phase is run till we cover all positives in the data using some solution rule or we exhaust all stages $k = 1,2,3,\ldots, n$ (whichever is reached first). The simplifiaction phase uses a greedy set cover to find a small subset of solution rules that still explain all the positives in the data. The greedy set cover algorithm is described in Algorithm \ref{alg:te2rules_simplification}. We start by selecting the rule that covers the most number of positives. Then, we remove these positives from the dataset and again the select the rule that has the highest coverage of positives that are left in the dataset. We repeat this process till no more positives are left in the dataset. We present the selected list of rules as an explanation to the user.
